# Supplementary material for: Unveiling Crowdfunding Futures: Analyzing Campaign Outcomes through Distributed Models and Big Data Perspectives
Source: arXiv:2402.14111 source file (2024-02-21)
Supplement: Supplementary file 1 [file Appendix.tex]

\section{Appendices} \label{sec:appendix}
\subsection{Platform} \label{sec:app_plat}
Kickstarter is a reward-based crowdfunding platform that was founded in 2009 and has had a substantial impact on society. In 2015, it transitioned into Kickstarter PBC, a Public Benefit Corporation. This change in its business model transformed it into a for-profit company with a legal obligation to consider the impact of its decisions on society, rather than solely on shareholders. As a result, Kickstarter PBC has additional legal obligations such as appointing specialized management, ensuring long-term sustainability, and transparent reporting of social outcomes achieved. In return, the company receives favorable tax treatment. Therefore, the success of meaningful campaigns is just as important as profitability, with Kickstarter earning a $5\%$ fee on successfully funded projects.

However, as it is not a non-profit organization, charitable donations or political financing are not part of its structure. Projects on Kickstarter are supported in exchange for rewards, often in the form of a prototype of the work or an exclusive experience such as a preview or personalized acknowledgment. These rewards cannot be direct monetary compensation, but they can provide indirect benefits (for example, a discount on a prototype or a ticket to a performance). Kickstarter does not claim ownership rights over the projects or the resulting works created.

Kickstarter does not provide guarantees regarding the actual use of funds by project creators, nor does it guarantee project completion or that the results will align with the expectations of backers. There is no quality control or feasibility assessment based on the requested funding amount. However, the platform encourages project creators to provide detailed explanations of their projects, both from a technical and financial standpoint. Kickstarter also supports both creators and backers through frequently asked questions (FAQ) lists. Not all creative projects can be supported on the platform (e.g., medical treatments, gambling, financial services, drugs, weapons, replicas of existing projects, etc.), and not everything can be offered as a reward (e.g., alcohol, live animals, resold items, etc.) see \href{https://www.kickstarter.com/rules/prohibited}{prohibited items list}.

Only adult citizens with a bank account and residing in a limited number of countries (including Italy since 2015) can present and create projects deemed "creative" on the platform. However, these projects can be funded from anywhere in the world.

The success of a project is determined by exceeding the funding goal, and in case of not reaching the goal, all backers are fully refunded. This approach, commonly known as "All or nothing," is widely used by platforms that focus on individual projects. The range of projects considered creative is highly diverse, spanning from films and short films to documentaries and music videos, from board games to digital games, from food to fashion, and also encompassing theater, dance, photography, comics, books, newspapers, art, design, and even technological products and technological tools for creating new original works (Note: There might not be campaigns specifically focused on AI for Arts, but it should be possible to initiate such projects). Once a project is created, it cannot be modified or removed from the website and remains permanently accessible to the public.

\subsection{variables}
\label{App:variables}
Below are some important observations regarding the nature of the variables introduced in Table \ref{tab:variables}:
\begin{enumerate}
    \item \textbf{ID}: The ID variable serves as a unique identifier for each observation, likely assigned based on the order of insertion. It acts as a primary key for referencing individual entries in the dataset. \rred{Potremmo rimuoverlo/sintetizzarlo}

    \item \textbf{name}: The name variable represents the name of the Kickstarter project for which a crowdfunding campaign is initiated. It provides a descriptive title or label for identifying different projects.

    \item \textbf{main\_category}: The main\_category variable indicates the primary category to which the crowdfunding campaign belongs. It helps classify campaigns into broader thematic groups.

    \item \textbf{category}: The category variable represents the subcategory to which the crowdfunding campaign belongs. It provides more specific information about the project's domain or theme within the main category.

    \item \textbf{launched}: The launched variable denotes the date and time when the campaign was officially launched on the Kickstarter platform. It provides a timestamp for the start of the fundraising period.

    \item \textbf{deadline}: The deadline variable represents the date when the crowdfunding campaign is scheduled to end. It signifies the cutoff point for accepting pledges and reaching the funding goal.

    \item \textbf{state}: The state variable indicates the current status of the campaign and can take on five possible values: 'suspended', 'failed', 'canceled', 'successful', or 'live'. It provides insights into the overall outcome or progress of the campaign.

    \item \textbf{backers}: The backers variable denotes the number of individuals who have supported the campaign by making financial contributions. It represents the count of backers at a specific point in time.

    \item \textbf{currency}: The currency variable indicates the currency in which the campaign's funding goals and financial transactions are denominated. It represents the preferred monetary unit chosen by project creators.

    \item \textbf{country}: The country variable represents the geographical location associated with the campaign. It identifies the country from which the campaign originates or is primarily targeted.

    \item \textbf{goal}: The goal variable represents the funding goal of the campaign, expressed in US dollars. It signifies the target amount that needs to be raised to achieve a successful campaign outcome.

    \item \textbf{usd\_goal\_real}: The usd\_goal\_real variable refers to the campaign's funding goal converted to US dollars using the \textit{Fixer.io} API. It provides a standardized measure of the funding goal in a common currency.

    \item \textbf{pledged}: The pledged variable represents the total amount of money pledged towards the campaign, expressed in US dollars. It indicates the cumulative financial support received throughout the campaign or at its conclusion.

    \item \textbf{usd\_pledged}: The usd\_pledged variable denotes the amount pledged towards the campaign converted to US dollars by Kickstarter. It provides a standardized measure of the pledged amount in a common currency.

    \item \textbf{usd\_pledged\_real}: The usd\_pledged\_real variable signifies the amount pledged towards the campaign converted to US dollars using the \textit{Fixer.io} API. It represents a standardized measure of the pledged amount in a common currency.
\end{enumerate}
